# Supplementary material for: Contests to Incentivize a Target Group
Source: arXiv:2204.14051 source file (2022-04-29)
Supplement: Supplementary file 3 [file additional.tex]

\section{Additional Topics}
\abheek{These additional topics, like maximizing total effort or allocation of prizes to the target group, can be added if it seems relevant. Will take advise from Edith and Paul on what to do.}

\subsection{Maximizing Allocation of Prize to a Group}
In this section, we study the amount of prize that is allocated to the players in the first group. Note that $\beta(v)$ is a monotonically increasing function in $v$, so the ranking of the players is directly determined by their abilities. For the contest that awards the entire prize to the first ranked player, the expected amount of prize awarded to players in the first group is equal to the probability that the winner is in the first group. This probability can be computed as:
\begin{multline*}
    \bP[winner \sim F] = \sum_{i \in [n]} \bP[winner = i, i \sim F] = \sum_{i \in [n]} \bP[winner = i \mid i \sim F] \bP[i \sim F] \\
    = \alpha \sum_{i \in [n]} \bP[winner = i \mid i \sim F]
    % &= \alpha \sum_{i \in [n]} \int_0^1 H^{n-1}(v_i) dF(v_i) \\
    = \alpha n \int_0^1 H^{n-1}(v) dF(v),
\end{multline*}
where $i \sim F$ denotes player $i$ belongs to the first group (with distribution $F$).

In a similar manner, for a general rank-order prize allocation, we can compute the expected prize money awarded to players belonging to the first group as:
\begin{align*}
    \bE[\text{prize awarded to players $\sim F$}] &= \sum_{i \in [n]} \sum_{j \in [n]} w_j \bP[\text{player $i$ gets rank $j$}, i \sim F] \\
    &= \alpha \sum_{i \in [n]} \sum_{j \in [n]} w_j \bP[\text{player $i$ gets rank $j$} \mid i \sim F] \\
    &= \alpha n \sum_{j \in [n]} w_j \int_0^1 p^H_j(v) dF(v) \\
    &= \alpha n \sum_{j \in [n]} w_j \int_0^1 h_{n,j}(v) \frac{f(v)}{h(v)} dv. \\
\end{align*}
Note that we have assumed that the prizes are non-increasing $w_j \ge w_{j+1}$; this is essential to have an well-behaved equilibrium where the output $\beta(v)$ is monotonically increasing in ability.

From the analysis above, we see that the optimal contest if again a simple contest that distributes the prize among first $k$ players, where $k$ is given by:
\[ k = \argmax_{l \in [n]} \sum_{j \in [l]}\frac{1}{l} \int_0^1 h_{n,j}(v) \frac{f(v)}{h(v)} dv. \]

The extreme cases: if $\frac{f(v)}{h(v)}$ is an increasing function, then it is optimal to allocate the prize to the first-ranked player, because $\int_0^1 h_{n,j}(v) dv = 1$ for every $j$ and $h_{n,j}(v)$ is single-crossing w.r.t. $h_{n,l}(v)$ for $l > j$; if $\frac{f(v)}{h(v)}$ is a decreasing function, we should distribute the prize equally among all $n$ players, which leads to no competition and zero output from every player; if $\frac{f(v)}{h(v)} = constant$ (where $constant$ must be $1$), then any prize allocation scheme is equivalent as $\int_0^1 h_{n,j}(v) dv = 1$ for every $j$.

In general, the shapes of $h_{n,j}(v)$ and $\frac{f(v)}{h(v)}$ together determines the optimal contest, where $\int_0^1 h_{n,j}(v) \frac{f(v)}{h(v)} dv$ is the inner-product between the two functions, and therefore captures similarity between them. The function among $\left( \sum_{j \in [l]} \frac{1}{l} h_{n,j}(v) \right)_{l \in [n]}$ that is most similar to $\frac{f(v)}{h(v)}$ is selected.
